# Supplementary material for: Learning Self-Regularized Adversarial Views for Self-Supervised Vision Transformers
Source: arXiv:2210.08458 source file (2022-10-16)
Supplement: Supplementary file 1 [file appendix.tex]

\textbf{Longer Training and Different Architecture.} We perform experiments on more settings (i.e., 400, 800 epochs and ViT-B). The results are shown in \cref{tab:longer train}. AutoView consistently improves the performance of ViTs on different training epochs and architectures. And the \cref{fig:improvements} intuitively shows our continuous boost on different training lengths. 

% We observe in \cref{tab:longer train} that AutoView consistently improves DINO in longer training of 800 epochs by 0.4\% $k$-NN classification accuracy. And the \cref{fig:improvements} intuitively shows our continuous boost on different training lengths.

\textbf{Fine-Tuning on ImageNet-1K.} 
% We study the fine-tuning on ImageNet-1K. $Rand.$ denotes the supervised baselines reported in \cite{touvron2021deit}. As shown in \cref{tab:fine-tune}, AutoView achieves 81.9\% and 82.9\% top-1 accuracy with ViT-S/16 of 800 epochs and ViT-B/16 of 400 epochs pre-training, yielding a performance gain of 0.4\% and 0.1\% compared to the baseline respectively. 
We study the fine-tuning on ImageNet-1K. $Rand.$ denotes the supervised baselines reported in \cite{touvron2021deit}. As shown in \cref{tab:fine-tune}, AutoView achieves 81.9\%  top-1 accuracy with ViT-S/16 of 800 epochs pre-training, 
yielding a performance gain compared to the baseline. 
% yielding a performance gain of 0.4\% compared to the baseline. 

\begin{table}[ht]
    \footnotesize
    \centering
    \begin{tabular}{lccc}
    \toprule
      Method & Arch  & epoch  & Acc \\\midrule
      \textcolor{gray!80}{Rand.} & \textcolor{gray!80}{ViT-S/16} & \textcolor{gray!80}{-} & \textcolor{gray!80}{79.9} \\
%    DINO& ViT-S/16 & 300 & 81.3\\ % 81.35 81.29
     DINO Manual& ViT-S/16 & 800 & 81.5\\ % 82.0
    
% \rowcolor{mypink} AutoView & ViT-S/16 &300 & \textbf{81.5}\\% 81.53 81.6
\rowcolor{mypink}DINO AutoView & ViT-S/16 &800 & \textbf{81.9}\\ % 81.92
% \midrule
%  \textcolor{gray!80}{Rand.} & \textcolor{gray!80}{ViT-B/16} & \textcolor{gray!80}{-} & \textcolor{gray!80}{81.8} \\
%  DINO Manual& ViT-B/16 & 400 & 82.8\\ % 83.6
%  \rowcolor{mypink}DINO AutoView & ViT-B/16 &400 & \textbf{82.9} \\
 \bottomrule
    \end{tabular}
    \caption{Fine-tuning on ImageNet-1K.}
    \label{tab:fine-tune}
\end{table}
